# Supplementary material for: Nonlinear erasing of propagating spin-wave pulses in thin-film Ga:YIG
Source: arXiv:2311.17821 ancillary file (2024-02-01)
Supplement: Supplementary file 1 [file 20240201_Supplementary_SW_Erasing.pdf]

## Supplemental Material

-

# Nonlinear erasing of propagating spin-wave pulses in thin-film Ga:YIG


D. Breitbach,[1,a)] M. Bechberger,[1,a)] B. Heinz,[1] A. Hamadeh,[1] J. Maskill,[1] K. O. Levchenko,[2] B. Lägel,[1] C. Dubs,[3] Q. Wang,[4] R. Verba,[5] and P. Pirro[1]

[1)] *Fachbereich Physik and Landesforschungszentrum OPTIMAS, Rheinland-Pfälzische Technische Universität Kaiserslautern-Landau, D-67663 Kaiserslautern, Germany*

[2)] *Faculty of Physics, University of Vienna, Boltzmanngasse 5, A-1090 Wien, Austria*

[3)] *INNOVENT e.V. Technologieentwicklung, D-07745 Jena, Germany*

[4)] *School of Physics, Huazhong University of Science and Technology, 430074 Wuhan, China*

[5)] *Institute of Magnetism, Kyiv 03142, Ukraine*

(*Electronic mail: dbreitba@rptu.de)



(Dated: 1 February 2024)


[a)] D. Breitbach and M. Bechberger contributed equally to this work.

## Contents


I. Thermal spin-wave spectrum 3

II. Excitation efficiency of the coplanar waveguide 4

III. Microwave excitation for group velocity measurements 4

IV. Role of the excitation frequency and field in the experiment 5

V. Decay of propagating spin waves 7

VI. Erasing process of the slow spin-wave pulse in the time domain 8

VII. Micromagnetic simulations 9

# I. Thermal spin-wave spectrum

This section provides additional information on the magnetic configuration of the Ga:YIG thin film with respect to the chosen external magnetic bias field.

In Fig. S1, the frequency-resolved BLS intensity of the thermal spin-wave population is shown as a function of the applied in-plane bias field $\mu_0 H_{\mathrm{app}}$. The detected thermal signal corresponds, in good approximation, to the FMR frequency of the system. In remanence or at low fields, the static magnetization points out-of-plane due to the perpendicular magnetic anisotropy, and since the BLS spectroscopy is not sensitive to this configuration, no thermal spin-wave signal is detected. As the external field is further increased, the static magnetization is tilted towards the in-plane direction, increasing the BLS sensitivity and rendering the thermal spin-wave signal detectable. This signal decreases with increasing field until it reaches a minimum, from which it increases again. The theoretical description of the FMR frequency for the in-plane magnetized geometry is given by[1]

$$\omega_{\mathrm{FMR}} = \gamma \mu_0 \sqrt{H_{\mathrm{app}}(H_{\mathrm{app}} + M_{\mathrm{eff}})}, \tag{S1}$$

with the gyromagnetic ratio $\gamma$ and the effective magnetization $\mu_0 M_{\mathrm{eff}} = \mu_0 M_{\mathrm{S}} - \mu_0 H_{\mathrm{U}} = -73.9\,\mathrm{mT}$[2]. Since $M_{\mathrm{eff}}$ is negative, the expression is not defined for an applied field value smaller than this. This field value is known as the compensation point, above which the magnetization can be approximated to point in the film plane. This was also considered by Carmiggelt *et al.*[3] who calculated the angle of the static magnetization using a more general description. In all of the

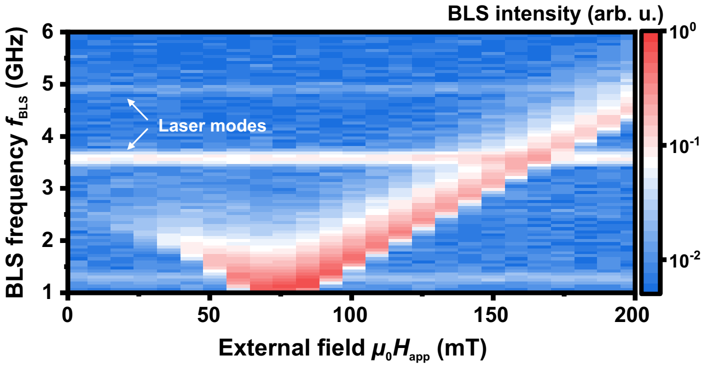


FIG. S1. Thermal BLS spectrum as a function of the applied in-plane field. Two horizontal modes are observed in the spectrum which are emitted by the probing laser, and, as a consequence are unrelated to the spin-wave signals.

discussed measurements, a magnetic field value $\mu_0 H_{app} \approx 85\,\mathrm{mT}$ was selected that is above the compensation point to ensure an in-plane configuration.

## II. Excitation efficiency of the coplanar waveguide

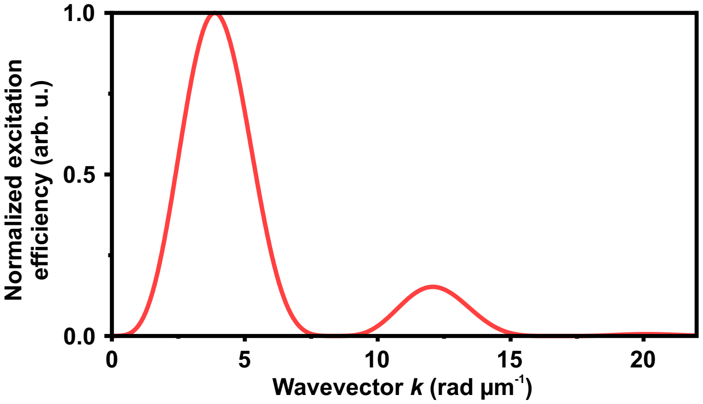


FIG. S2. Normalized excitation efficiency of the CPW antenna of Fig. 1 of the main manuscript.

The excitation efficiency of the coplanar waveguide is strongly dependent on the wavevector of the excited spin-wave. It is proportional to the spatial Fourier transform of the magnetic Øersted field generated by the alternating electric current flowing through the CPW antenna[4]. As BLS detects the spin-wave intensity and not amplitude, the square of this value was calculated, which is shown in Fig. S2. This factor is sufficient as an estimation of the accessible wavevectors in our experiment.

## III. Microwave excitation for group velocity measurements

This section provides additional information on the choice of microwave powers for the group velocity measurements (Fig. 2 in the main manuscript). As discussed in the previous section, the excitation efficiency of the CPW antenna depends on the excited wavevector (frequency). In addition, depending on the configuration of the external magnetic field, $\mathbf{k} \parallel \mathbf{H}_{app}$ or $\mathbf{k} \perp \mathbf{H}_{app}$, either one or two dynamic Øersted field components of the CPW exert a torque on the magnetization. The powers chosen for these four configurations therefore differ and each resembles a trade-off between the signal-to-noise ratio and the impact of nonlinear effects. This regime was determined by measuring the BLS intensity of the pulses as a function of the excitation power, see Fig. S3.

The power was chosen well below the saturation level of the intensity which indicates an onset of strong nonlinearities, see Fig. S3 and Tab. S1.

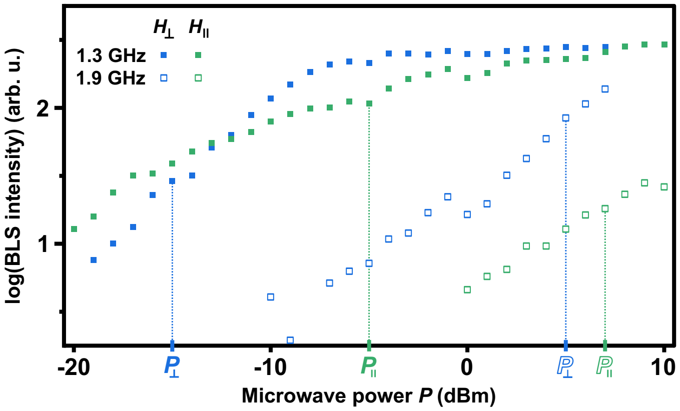


FIG. S3. BLS intensity of the spin-wave pulse as a function of the applied microwave power. The measurement was performed for two frequencies $f = 1.3\,\text{GHz}$ and $f = 1.9\,\text{GHz}$, representing the two maxima in excitation efficiency, respectively, and for two field configurations. The chosen power levels are marked by vertical lines. Parameters: $\mu_0 H_\perp = 88.54\,\text{mT}$ and $\mu_0 H_{||} = 85.76\,\text{mT}$, position: $x \approx 3\,\mu\text{m}$.

TABLE S1. Power levels used in Fig. 2 in the main manuscript.

| | $P_\perp$ (dBm) | $P_{||}$ (dBm) |
|---|---|---|
| first CPW maximum | -15 | -5 |
| second CPW maximum | 5 | 7 |

## IV. Role of the excitation frequency and field in the experiment

This section explains in more detail the choice of the excitation frequencies $f_\mathbf{A} = 1.11\,\text{GHz}$ and $f_\mathbf{B} = 2.2\,\text{GHz}$ and the applied magnetic field $\mu_0 H_\text{app}$ for the observation of the erasing effect. While the frequency of the slow pulse $f_\mathbf{A}$ should be close to the minimal frequency of the spin-wave spectrum, the choice of a factor of almost two between the excitation frequencies is not crucial for the observed phenomenon, as three-magnon decay is prohibited in a thin film with in-plane static magnetization. Thus, the frequency of pulse **B** can, in principle, be varied, as is demonstrated using micromagnetic simulations (see Sec. VII). Ideally, $f_\text{B}$ would be as high as possible to maximize the group velocity of pulse **B** following the almost linear relation $v_\text{G}(k) \propto k$. There are,

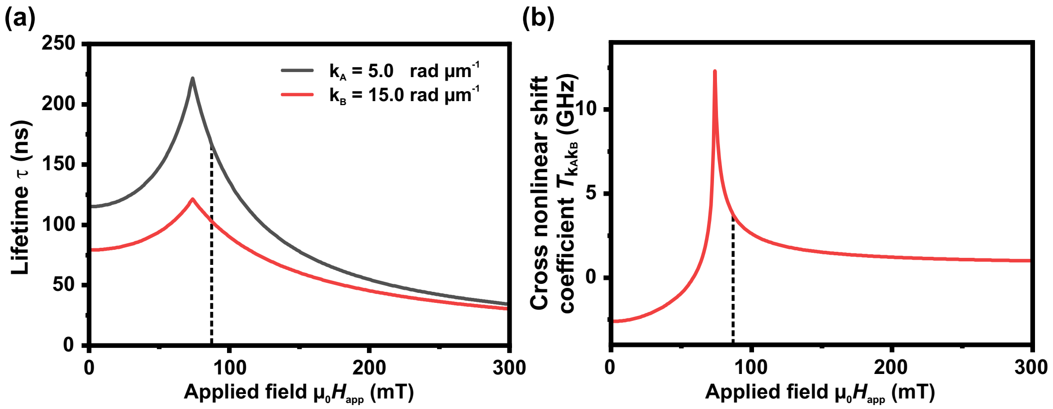


FIG. S4. Calculation of **(a)** the spin-wave lifetime $\tau$ and **(b)** the cross nonlinear frequency shift coefficient $T_{\mathbf{k_A k_B}}$ as a function of the applied magnetic field $\mu_0 H_{\mathrm{app}}$. The pronounced spike arises due to the compensation point, at which the magnetization changes from out-of-plane to in-plane configuration. The calculations were performed for the material parameters given in the manuscript.

however, several experimental limitations to consider. When moving to higher wavevectors at a given field, the excitation efficiency of the CPW antenna (see Sec. II) decreases with increasing wavevector $k$. Also, the BLS detection efficiency decreases towards higher wavevectors, which is a rather technical difficulty.

In terms of the applied field, the eraser effect is principally not limited to the specific value used in the main manuscript. When varying the field, however, it is important to take into account the following dependencies. First, the spin-wave lifetime $\tau$ significantly decreases with increasing field, see Fig. S4 **(a)**. This reduces the spin-wave decay length which increases the required excitation power for pulse **B**. Second, the cross nonlinear frequency shift coefficient $T_{\mathbf{k_A k_B}}$ has a field dependence, see Fig. S4 **(b)**. While its value close to the compensation point is high, it strongly decreases towards higher applied field values. Note that the maxima in Fig. S4 **(a)** and **(b)** are related to the compensation point.

In summary, the mechanism of the erasing effect is principally robust against a change of field and frequency $f_{\mathrm{B}}$, as long as $f_{\mathrm{A}}$ is close to the band bottom and $T_{\mathbf{k_A k_B}}$ is positive. Our micromagnetic simulation in Fig. S8 **(b)** demonstrates that the effect can even be observed even at $f_{\mathbf{B}} = 2.5\,\mathrm{GHz}$. The experimental realization, however, might be more difficult due to a changed spin-wave lifetime or excitation efficiency, or nonlinear coefficient.

## V. Decay of propagating spin waves

The evolution of the measured intensity of the pulses along the propagation length (see Fig. 2 in the main manuscript) appears different for the pulses **A** and **B**. While pulse **A** shows a pronounced decay, pulse **B** does not show a clear trend in intensity decay. This is attributed to the inherent properties of the signal, i.e., the mode $k_{\mathbf{B}}$ has a decay length much larger than the measurement scan length.

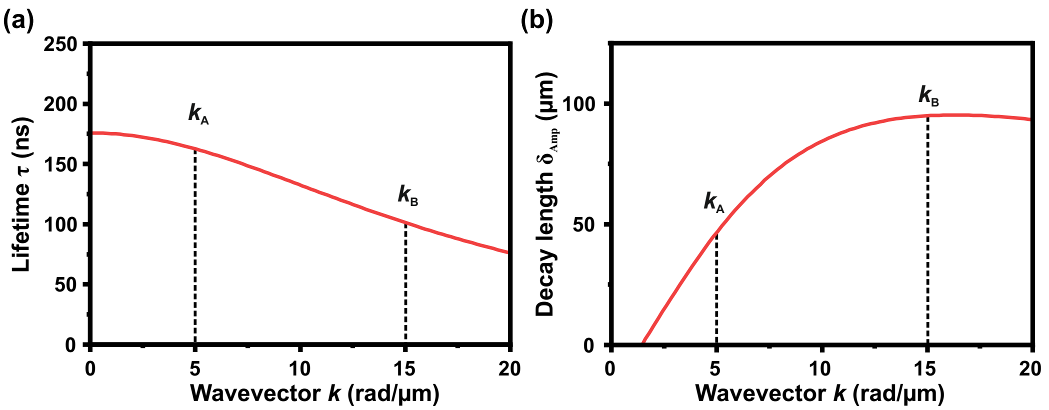


FIG. S5. **(a)** Calculated spin-wave lifetime and **(b)** spin-wave amplitude decay length as a function of the wavevector. The wavevectors of pulse **A** and pulse **B** are marked by dashed lines. Calculated for $\mu_0 H_{\text{app}} = 86\,\text{mT}$ and the material parameters given in the manuscript.

Figure S5 shows a theoretical analysis of the spin-wave lifetime and decay length as a function of the wavevector, following the standard approach $\tau = (\alpha\omega\frac{\partial\omega}{\partial\omega_{\text{H}}})^{-1}$ and $\delta = \tau \cdot v_{\text{G}}$. It reveals that spin-wave mode $k_{\mathbf{B}}$ has a decay length substantially longer than mode $k_{\mathbf{A}}$ and than the length of our measurement. This is due to the fact that, despite its shorter lifetime, mode $k_{\mathbf{B}}$ has a considerably higher group velocity than mode $k_{\mathbf{A}}$ (see Fig. 2 in main manuscript). This reflects in the amplitude decay length $\delta_{\mathbf{B}} = 95\,\mu\text{m}$ shown in Fig. S5 **(b)** which is approximately twice as high as $\delta_{\mathbf{A}} = 47\,\mu\text{m}$. The observation that a pronounced decay is still observed for pulse **A** likely stems from the fact that wavevectors $k < 5\,\text{rad}\,\mu\text{m}^{-1}$ have much shorter decay lengths. These are partially excited within the frequency linewidth of the excitation due to the very flat spin-wave dispersion at low wavevectors.

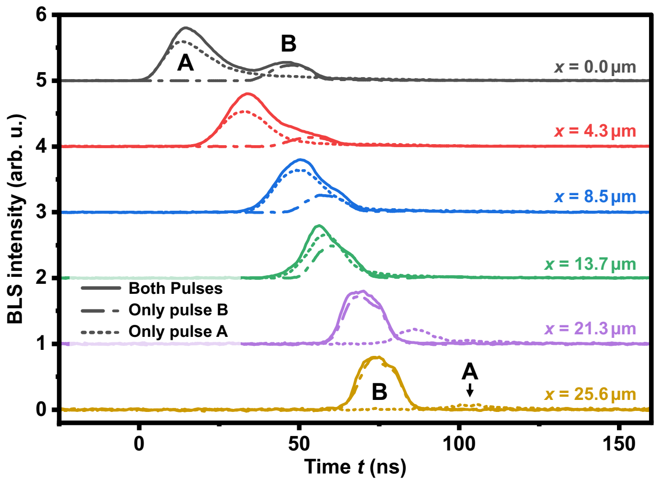


FIG. S6. Time-dependent BLS intensities at several measurement positions (data from Fig. 3 in the main manuscript), all of which are separated by intensity offsets in increasing levels of +1 for clarity. Two scenarios are shown: The interacting case (both pulses are excited, solid line) and the non-interacting case (pulse **A** and pulse **B** are excited separately, dashed lines). Differences between those scenarios highlight that nonlinear interaction takes place. Parameters: $P_\mathrm{A} = 0\,\mathrm{dBm}$ and $P_\mathrm{B} = 15\,\mathrm{dBm}$, applied field $\mu_0 H_\mathrm{app} = 86\,\mathrm{mT}$.

## VI. Erasing process of the slow spin-wave pulse in the time domain

In this section, we show additional time traces of the erasing process of the slow pulse **A**. Figure S6 depicts the time-dependent BLS intensities integrated over the BLS spectrum ($0.5 - 3.0\,\mathrm{GHz}$) at several measurement positions. Shown are the interacting case, i.e., when both pulses are excited (**solid lines**), and the non-interacting case, i.e., when only the individual pulses are excited (**dashed lines**). For better illustration, an artificial offset of $+1$ is included for each subsequent measurement position and they are each normalized to their highest intensity to show their fine details despite the exponential spin-wave decay. In the non-interacting case, it is apparent that the time-delayed, faster pulse **B** can easily catch up with pulse **A**, and would overtake it until they would be completely separated in space and time. In the interacting case however, pulse **A** is not visible anymore after being passed by pulse **B** even in positions where it was seen in the non-interacting case.

Fig. S7 shows the erasing of pulse **A** through pulse **B** for different powers $P_\mathrm{B}$ measured at a position immediately after the pulse crossing at $x = 20\,\mu\mathrm{m}$. When the microwave **B** is turned off,

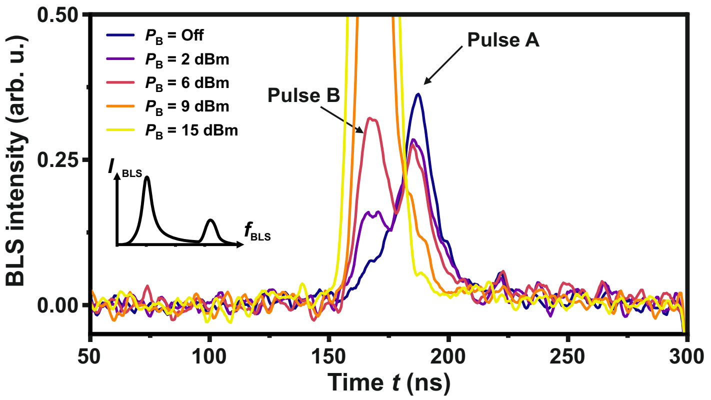


FIG. S7. Time-resolved BLS intensity, integrated over the BLS spectrum ($0.8-3.0\,\mathrm{GHz}$), showing the reconstruction of pulse **A** past pulse **B** for different excitation powers $P_\mathrm{B}$. Parameters: $x = 20\,\mu\mathrm{m}$, $P_\mathrm{A} = 0\,\mathrm{dBm}$, $\mu_0 H_\mathrm{app} = 86\,\mathrm{mT}$, $\mathbf{k} \perp \mathbf{M}$.

the undisturbed pulse **A** is visible. Once pulse **B** is also excited, it emerges shortly before pulse **A** in the intensity profile. With increasing power $P_\mathrm{B}$, the intensity of pulse **B** increases, while pulse **A** decreases until it is completely erased. Compared to Fig. 4 in the main manuscript, where only BLS frequencies around $f_\mathrm{BLS} = 1.11\,\mathrm{GHz}$ were shown to isolate the attenuation effect, here an integration over the whole spectrum is plotted.

## VII. Micromagnetic simulations

Micromagnetic simulations were performed utilizing the Mumax3 micromagnetic solver[5]. These simulations were designed to provide a comparative analysis to our experimental results and were performed for similar material and field parameters as the experiment. Please find the exact simulation parameters at the end of this section.

In the simulation, an excitation width of 200 nm was used, allowing for the excitation of higher spin-wave frequencies compared to the experiment. The frequency of pulse **A** was set to $f_\mathbf{A} = 1.11\,\mathrm{GHz}$ at a fixed excitation amplitude. In the case of pulse **B**, two distinct frequencies were explored which can be observed in Fig. S8: **(a)** $f_\mathbf{B} = 2.2\,\mathrm{GHz}$ and **(b)** $f_\mathbf{B} = 2.5\,\mathrm{GHz}$. All color plots in Fig. S8 share the same normalization and color scale. The amplitude $\mu_0 h_\mathbf{B}$ of the excitation field was methodically varied from top to bottom panels, starting from the absence of pulse **B**, progressing through a linear superposition with pulse **A**, and lastly resulting in the nonlinear erasing of pulse **A**.

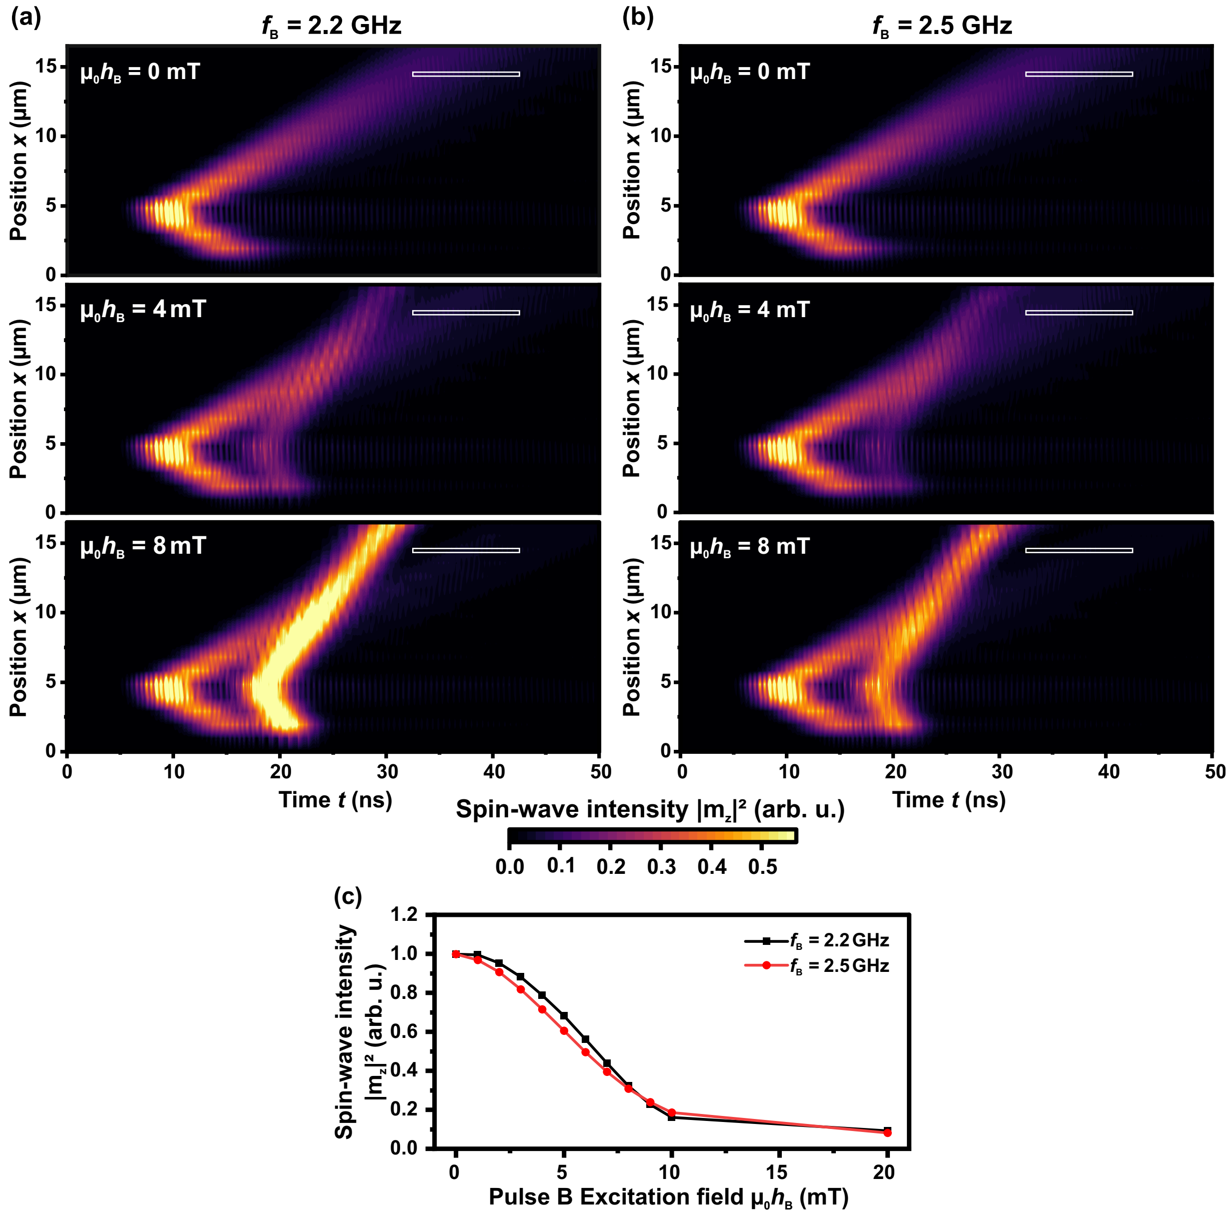


FIG. S8. Micromagnetic simulation of the nonlinear erasing experiment. For pulse **A**, a frequency of $f_\mathbf{A} = 1.11\,\text{GHz}$ and fixed excitation amplitudes were used. Pulse **B** was simulated with two different frequencies. **(a)** Spin-wave intensity $|m_z|^2$ as a function of position and time for $f_\mathbf{B} = 2.2\,\text{GHz}$ and **(b)** for $f_\mathbf{B} = 2.5\,\text{GHz}$ for increasing excitation field amplitude $\mu_0 h_\mathbf{B}$ from top to bottom. **(c)** The spin-wave intensity was averaged over a $100\,\text{nm} \times 10\,\text{ns}$ wide rectangle (white). The resulting signal of pulse **A** is depicted as a function of the pulse **B** excitation field.

To quantify the effect, the remaining intensity of pulse **A** was extracted after the crossing with pulse **B**. The spin-wave intensity was averaged over all cells in a $100\,\text{nm} \times 10\,\text{ns}$ region (indicated

as white rectangles). The result is shown in Fig. S8 **(c)** as a function of the pulse **B** excitation field $\mu_0 h_\mathbf{B}$. For both frequencies, a decline of the initial intensity of pulse **A** is observed for increasing amplitudes $\mu_0 h_\mathbf{B}$ until pulse **A** is almost fully erased.

In conclusion, the micromagnetic simulations are in good agreement with the experimental results and provide a more comprehensive understanding of the nonlinear erasing effect beyond the frequency range accessible in our experiment.

**Simulation parameters**: Structure size: $20000 \times 5000 \times 59\,\mathrm{nm}^3$, cell size: $c_\mathrm{x} = 9.77\,\mathrm{nm}$, $c_\mathrm{y} = 9.77\,\mathrm{nm}$, $c_\mathrm{z} = 59\,\mathrm{nm}$, saturation magnetization $M_\mathrm{S} = 1.6 \times 10^4\,\mathrm{A\,m^{-1}}$, exchange constant $A = 1.37\,\mathrm{pJ\,m^{-1}}$, uniaxial anisotropy constant $K_\mathrm{u1} = 94.1\,\mathrm{mT} \times M_\mathrm{S}/2$ pointing in the $z$-direction, temperature $T = 300\,\mathrm{K}$ and Gilbert damping parameter $\alpha = 6.1 \times 10^{-4}$. In our simulations, the Gilbert damping parameter was set to increase at the end of the device to avoid spin-wave reflection. An external field $\mu_0 H_\mathrm{app} = 86\,\mathrm{mT}$ was applied along the in-plane axis (y-direction) which is sufficient to magnetize the structure in the film plane. Periodic boundary conditions were applied in the $y$-direction. To excite a propagating spin-wave pulse, we applied a sinusoidal magnetic field with a Gaussian pulse envelope $b_z = b\sin(2\pi f t)\exp(-((t-t_0)/\sigma)^2)$ $5\,\mu\mathrm{m}$ from the center of the film in $x$-direction. The excitation field is applied over an area of 200 nm in $x$-direction and over the full film length in $y$-direction. The excitation field amplitude is in the range of $0-20\,\mathrm{mT}$, the excitation parameters are $f_\mathbf{A} = 1.11\,\mathrm{GHz}$, $f_\mathbf{B} = 2.2\,\mathrm{GHz}$ or $f_\mathbf{B} = 2.5\,\mathrm{GHz}$, $\sigma = 3\,\mathrm{ns}$, $t_0^\mathrm{A} = 8\,\mathrm{ns}$ and $t_0^\mathrm{B} = 18\,\mathrm{ns}$. The $M_\mathrm{z}(x,y,t)$ of each cell was collected over a period of 50 ns and recorded in 100 ps intervals. The dynamic component $m_\mathrm{z}(x,y,t)$ was calculated for all cells via $m_\mathrm{z}(x,y,t) = M_\mathrm{z}(x,y,t) - M_\mathrm{z}(x,y,0)$, where $M_\mathrm{z}(x,y,0)$ corresponds to the groundstate. The spin-wave intensities were calculated by taking $|m_\mathrm{z}(x,y,t)|^2$.

## References


[1] I. S. Maksymov and M. Kostylev, Physica E: Low-dimensional Systems and Nanostructures **69**, 253 (2015).

[2] T. Böttcher, M. Ruhwedel, K. O. Levchenko, Q. Wang, H. L. Chumak, M. A. Popov, I. V. Zavislyak, C. Dubs, O. Surzhenko, B. Hillebrands, A. V. Chumak, and P. Pirro, Applied Physics Letters **120**, 102401 (2022).

[3] J. J. Carmiggelt, O. C. Dreijer, C. Dubs, O. Surzhenko, and T. van der Sar, Applied Physics Letters **119**, 202403 (2021).

[4]T. Schneider, A. A. Serga, T. Neumann, B. Hillebrands, and M. P. Kostylev, Phys. Rev. B **77**, 214411 (2008).

[5]A. Vansteenkiste, J. Leliaert, M. Dvornik, M. Helsen, F. Garcia-Sanchez, and B. Van Waeyenberge, AIP Advances **4**, 107133 (2014).
